# Supplementary material for: Sensitivity of Trapping Efficiency and Relative Permeability to Experimental Methodology in Laboratory Core Flooding
Source: arXiv:2505.09044 source file (2025-05-14)
Supplement: Supplementary file 1 [file appendix.tex]

Pressure data for the full experiment 

Saturation profiles for the reversed orientation?
